# Supplementary material for: Fast 4D-STEM-based phase mapping for amorphous and mixed materials
Source: arXiv:2507.17068 ancillary file (2026-08-25)
Supplement: Supplementary file 1 [file Supplementary_Information.pdf]

**Fast 4DSTEM-based phase mapping for amorphous and mixed materials: Supplementary Information**

A. Werbrouck, N. C. Paranamana, X. He, M. J. Young

**Software package**

The python library developed for this work is available on Github at https://github.com/awwerbro/ePDF.

**Additional figures and discussion**

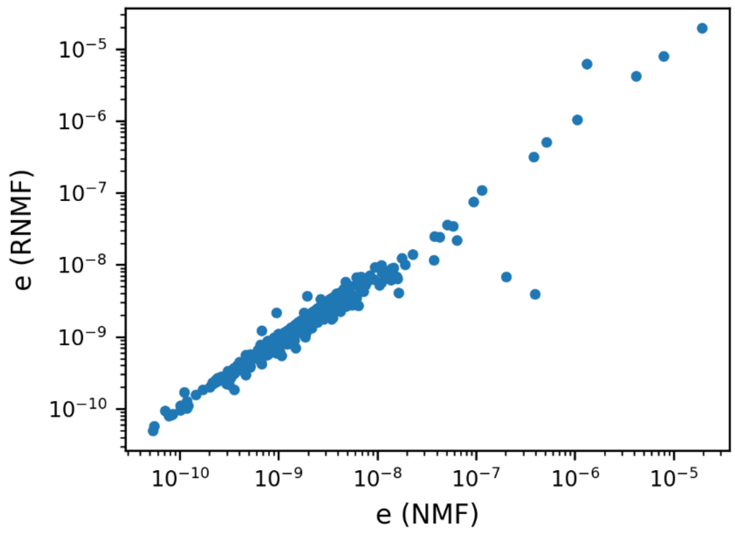


**Figure S1**: Average reconstruction errors per pixel for the full dataset as shown in Figure 3 (with a convergence criterion of $10^{-5}$). This data shows that the speedup offered by RNMF does not result in a loss of quality.

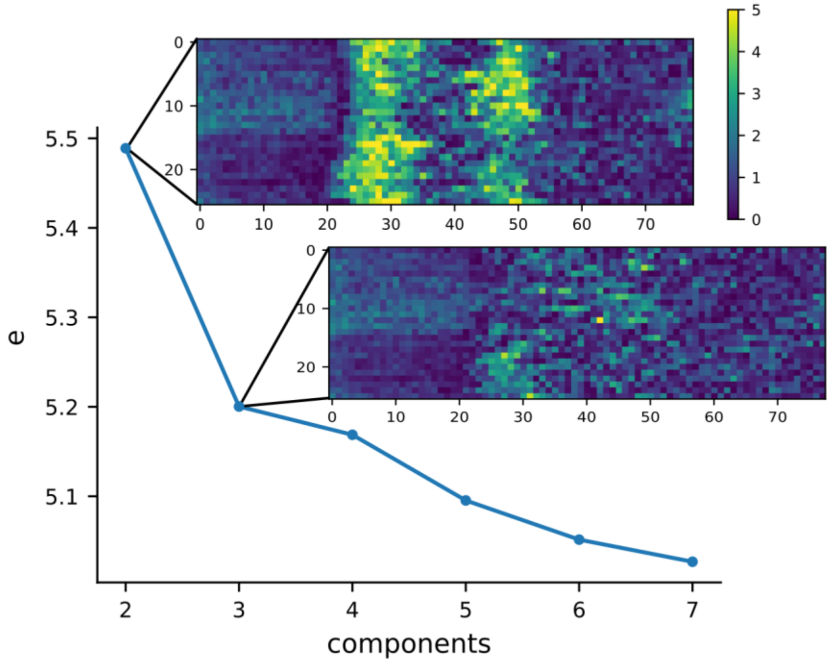


**Figure S2:** Sum of the reconstruction error as the number of components is increased for the TiO2 shell, and map of the residual for 2 and 3 components. The map for 2 components shows a clear local structure at the edge of the $TiO_2$ layer, which vanishes as we use 3 components. The color bar is the same for both maps.

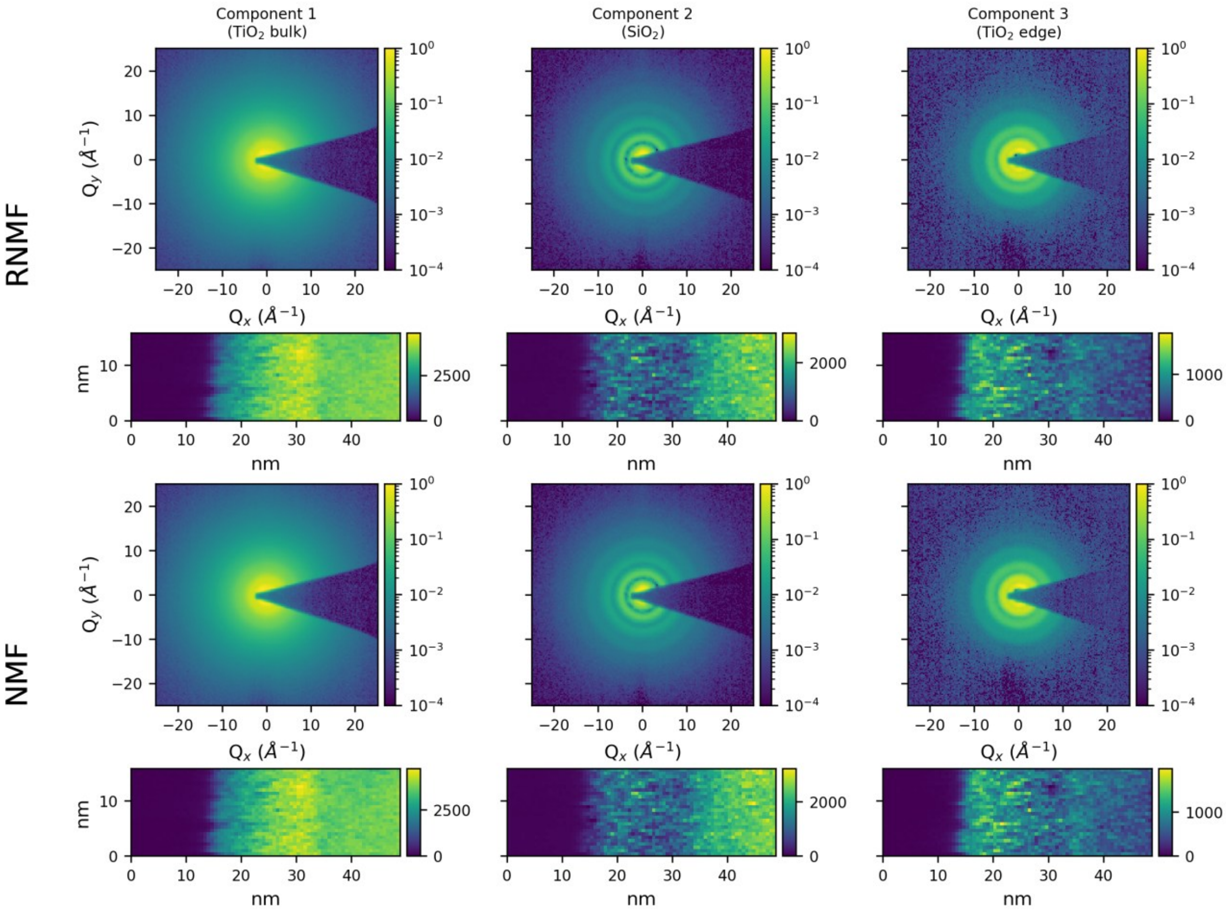


**Figure S3**: Comparison of components of factorization of dataset 1 into 3 components with RNMF and NMF. Results are near-identical.

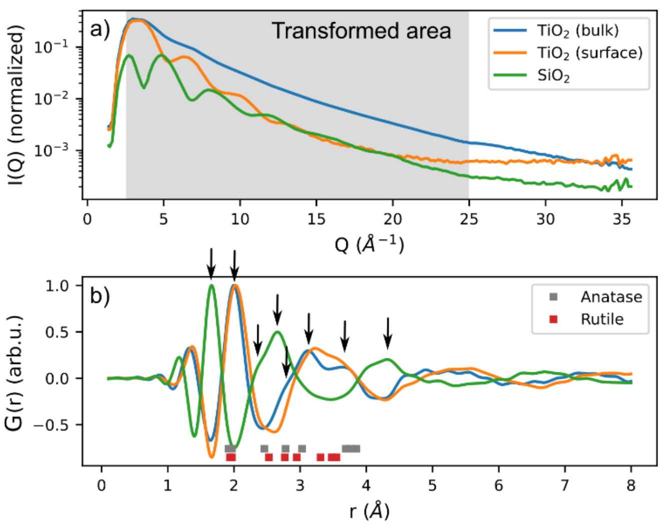


**Figure S4.** PDF analysis of RNMF components including (a) azimuthally integrated diffraction rings (components W) where the grey box indicates the data that was used to construct the PDFs and (b) normalized PDFs (G(r)) calculated for each component from the data in panel (a). There is a marked difference between $SiO_2$ and the $TiO_2$ components, but also $TiO_2$ shows subtle differences between bulk and surface components, indicating a lower density at the interface. Arrows indicate the position of the components described in the text. Expected peak positions for the crystalline rutile and anatase phases of $TiO_2$ are indicated.

**PDF analysis of $TiO_2$ and $SiO_2$**

The residual $r_{reciprocal}$ is displayed in Figure 4g, and the spatial map of the residual $r_{real}$ is displayed in Figure 4h, which shows that the error is close to the noise level. This indicates that a distinct structure may exist at the outer $TiO_2$ surface and at the interface between the $TiO_2$ and $SiO_2$.

Deeper insights into these structures are revealed upon further PDF analysis. Each 2D diffraction signal component depicted in Figure 4 a,c, and e was integrated azimuthally as presented in Figure S4a, and PDFgetX3 software used the 1D diffraction data between Q=2.5A-1 - 25A-1 to obtain a density-scaled reduced pair distribution function $G(r)/4\pi\rho_0$ for each component, as depicted in Figure S4b. The PDFgetX3 software models the scattering background as a polynomial, and values of the 'rpoly' parameter were 1.78, 1.84 and 1.74, for $TiO_2$ bulk, $SiO_2$, and $TiO_2$ interface respectively (See Figure S5). These values are within reasonable bounds.

Looking at the actual peaks in G(r), the obtained G(r) functions for each component match expectations based on literature for our expected assignments for the different components to $TiO_2$ and $SiO_2$. In vitreous $SiO_2$ [1] the coordination of Si is four-fold with Si-O bonds at 1.62Å, the OO distance is 2.65Å, Si-Si is 3.12, 4.15 (Si- 2nd O), 5.1Å, superposition of O-2nd O and Si-2nd Si. Disregarding the first, spurious peak at 1.15 Å (see below), the maxima of the G(r) obtained in this work are 1.65, (2.35), 2.65, (4.0), 4.31 Å, with the values within parentheses signifying 'shoulders'.

This indicates agreement up to the first/second coordination sphere, where discrepancies may arise because of different angle distributions.

For $TiO_2$, the distance of the first coordination sphere depends strongly on the crystal/amorphous phase and ranges from 1.8 to about 2.3Å [2], again depending on the bond angle distribution. Ignoring again the very first peak at 1.31Å, we find bulk peaks at 2.00, (2.8), 3.10, 3.67 A for bulk $TiO_2$, which can ascribe to Ti-O, (O-O) and Ti-Ti bonds respectively (with the Ti-Ti bonds responsible for the two last peaks). For the surface/interface $TiO_2$}, we find peaks at 2.02, (2.90), 3.22 and 3.53 Å, signifying that the surface/interface phase is less dense than the bulk $TiO_2$.

As we can explain the O-O, Si-O, Si-Si bonds (and Ti analogs) with these measurements, there is no suitable candidate to explain the peaks between 1 and 1.5 Å (1 peak per spectrum). One potential candidate would be OH-bonds, but the O-H bond length in Si-O-H is 0.969 Å [3] with similar values for Ti -O-H. Another option are Ti-Cl bonds (For $TiO_2$) which have a length of 2.18Å [4]. Additionally, the scattering cross-section of H is low. As such we interpret this peak as an artefact of the data processing. To substantiate this interpretation, Figure S5 shows the effect of background modeling in more detail. It is clear that the first peak in all 3 cases is highly dependent on the background model, while the other peaks remain constant.

The interatomic distances of the anatase and rutile phases are indicated in Figure S4b. The amorphous ALD film exhibits higher pair distances for all the key peak positions relative to the anatase and rutile phases (e.g. consider the second peak). We attribute this to a lower material density – where increases in the first and second coordination sphere pair distances indicate an expansion in the material volume, and therefore a lower density. It is known that the density of thin ALD films is generally lower than their PVD/larger scale counterparts and is temperature-dependent [5], [6]. The incorporation of H, leading to non-bridging oxygens is one potential explanation for this phenomenon, where the coordination of H to O will lengthen the adjacent Ti-O bonds[7].

We are not aware of previous reports describing a depth-dependent variation of density within ALD $TiO_2$ films. Our group has obtained results in the past for pair distribution measurements of ALD $Al_2O_3$ on CNTs [8], [9] where an undercoordinated surface structure of only a few Angstroms thickness was observed at the surface and interface. However, the surface reconstruction typically involved densification of the upper atomic layers, whereas here it seems as if the surface phase is of lower density and spans multiple nanometers (tens of atoms). From EDS measurements we could establish the presence of traces of Cl in the $TiO_2$ film, seemingly below the surface, in the phase we described as 'bulk' (Figure S6). This could point to post-deposition evaporation of HCl from the film, which may contribute to a less dense surface phase. However, the Cl signal is weak and may be below the detection limit in the outer shell of the sphere. It has also been reported that over significant timescales, amorphous $TiO_2$ films (deposited with a different precursor) can crystallize into the anatase phase [10]. The early stages of this transformation may be evident here. An alternative explanation could be the impact of the spherical geometry on temperature-induced strain, where post-deposition differences in thermal contraction could lead to different strain levels in the material at different radii producing different pair distances.

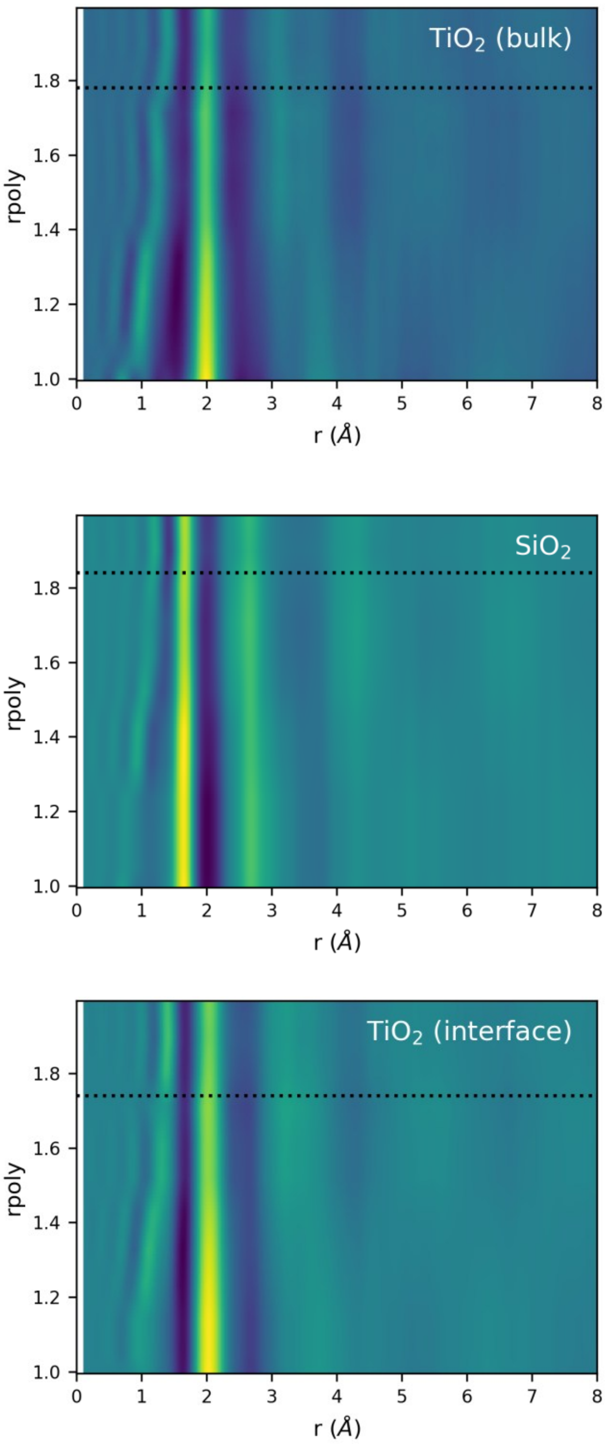


**Figure S5**: Analysis of the azimuthally integrated fingerprint spectra of respectively $TiO_2$ (bulk), $SiO_2$ and $TiO_2$ (interface) with PDFgetX3 shows that the first peak in the G(r) curves in Figure S4b is spurious and a result of the transformation from reciprocal space to real space. The heatmap shows the obtained G(r) for different values of the ‘rpoly’ parameter, used to model the background. The dotted line indicates the value that was used for the final analysis.

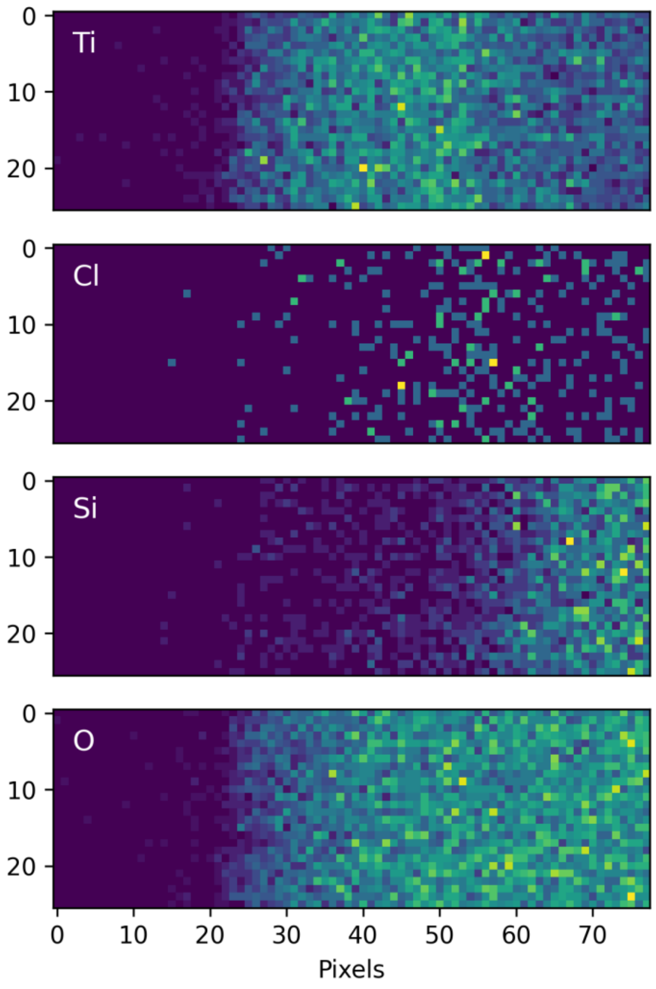


**Figure S6**: EDS data of the $TiO_2$ sample showing raw counts per cycle.

**PDF analysis of LGPS**

In Figure 5c, the first peak around 1.4 Å can be explained by the presence of S-O bonds, from O migrated through the sample. This is corroborated by an EDS map of a rather uniform O distribution (Figure S9). The second peak can be interpreted as a convolution of P-S (1.9Å [11], ~ 2.1Å [12], 2.0Å [13], Li-O [14] and Ge-S (2.4Å [15]).

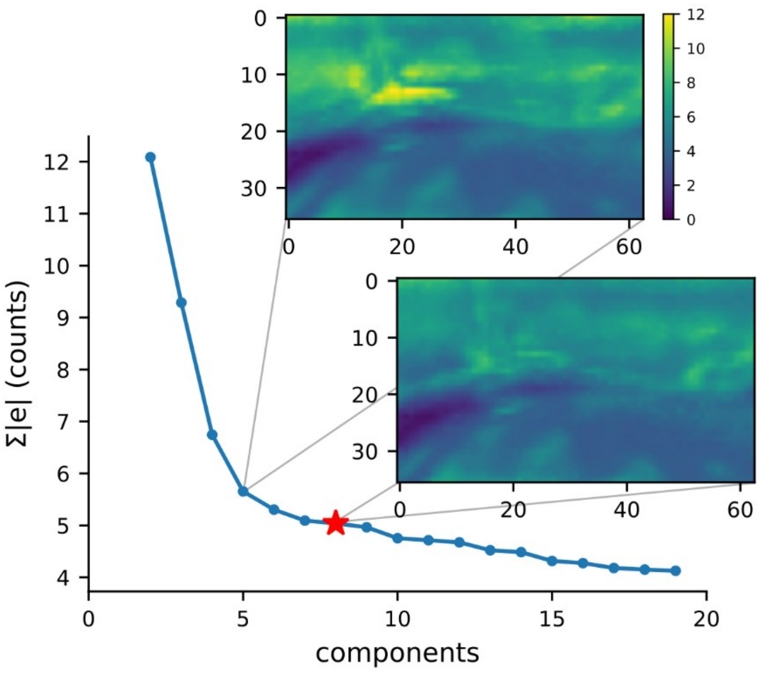


**Figure S7:** Sum of the reconstruction error as the amount of components is increased for the NMC-LGPS interface. The fact that there is some spatially correlated reconstruction error in the interface when 5 components are used in the 'elbow' of the error, led us to increase the amount of components to 8. As mentioned in the discussion, it is hard to quantify the amount of components when stress and/or strain are present, leading to continuous shifting of diffraction peaks.

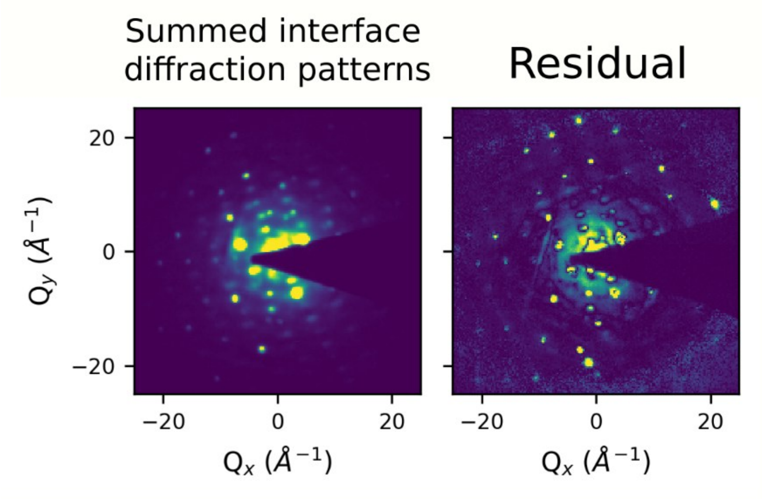


**Figure S8:** Sum of the components from figure 5c and residual diffraction images, noting the similarity between them. The residual map is displayed in Figure S7.

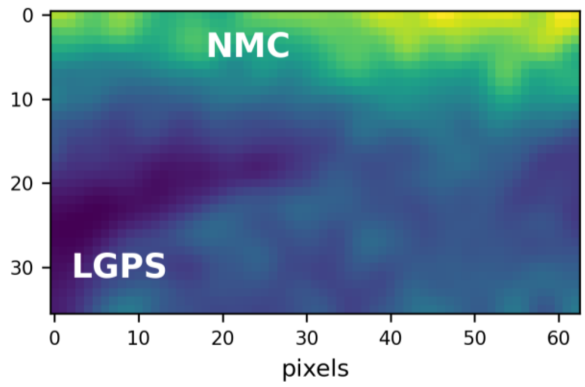


**Figure S9**: EDS map of O across the NMC-LGPS interface: while O has migrated to the LGPS region, its distribution in the LGPS region is relatively uniform, corroborating the NMF mapping of a single LGPS component.

## References


[1] R. L. Mozzi and B. E. Warren, “The structure of vitreous silica,” *Journal of Applied Crystallography*, vol. 2, no. 4, pp. 164–172, 1969, doi: 10.1107/S0021889869006868.

[2] J. Mavračić, F. C. Mocanu, V. L. Deringer, G. Csányi, and S. R. Elliott, “Similarity Between Amorphous and Crystalline Phases: The Case of TiO2,” *J. Phys. Chem. Lett.*, vol. 9, no. 11, pp. 2985–2990, Jun. 2018, doi: 10.1021/acs.jpclett.8b01067.

[3] M. C. McCarthy, F. Tamassia, D. E. Woon, and P. Thaddeus, “A laboratory and theoretical study of silicon hydroxide SiOH,” *The Journal of Chemical Physics*, vol. 129, no. 18, p. 184301, Nov. 2008, doi: 10.1063/1.3002914.

[4] None Available, “Materials Data on $TiCl_4$ by Materials Project.” LBNL Materials Project; Lawrence Berkeley National Laboratory (LBNL), Berkeley, CA (United States), 2020. doi: 10.17188/1204520.

[5] B. D. Piercy, C. Z. Leng, and M. D. Losego, “Variation in the density, optical polarizabilities, and crystallinity of TiO2 thin films deposited via atomic layer deposition from 38 to 150 °C using the titanium tetrachloride-water reaction,” *Journal of Vacuum Science & Technology A*, vol. 35, no. 3, p. 03E107, Mar. 2017, doi: 10.1116/1.4979047.

[6] M. E. DeCoster *et al.*, “Density and size effects on the thermal conductivity of atomic layer deposited $TiO_2$ and $Al_2O_3$ thin films,” *Thin Solid Films*, vol. 650, pp. 71–77, Mar. 2018, doi: 10.1016/j.tsf.2018.01.058.

[7] A. M. Jasim, X. He, Y. Xing, T. A. White, and M. J. Young, “Cryo-ePDF: Overcoming Electron Beam Damage to Study the Local Atomic Structure of Amorphous ALD Aluminum Oxide Thin Films within a TEM,” *ACS Omega*, vol. 6, no. 13, pp. 8986–9000, Apr. 2021, doi: 10.1021/acsomega.0c06124.

[8] M. J. Young *et al.*, “Probing the Atomic-Scale Structure of Amorphous Aluminum Oxide Grown by Atomic Layer Deposition,” *ACS Appl. Mater. Interfaces*, vol. 12, no. 20, pp. 22804–22814, May 2020, doi: 10.1021/acsami.0c01905.

[9] N. C. Paranamana, R. Gettler, H. Koenig, S. Montgomery-Smith, X. He, and M. J. Young, “Measuring Local Atomic Structure Variations through the Depth of Ultrathin (<20 nm) ALD Aluminum Oxide: Implications for Lithium-Ion Batteries,” *ACS Appl. Nano Mater.*, vol. 5, no. 9, pp. 12582–12591, Sep. 2022, doi: 10.1021/acsanm.2c02312.

[10] J. P. Wooding, K. Kalaitzidou, and M. D. Losego, “Crystalline as-deposited $TiO_2$ anatase thin films grown from TDMAT and water using thermal atomic layer deposition with in situ layer-by-layer air annealing,” *Atomic Layer Deposition*, vol. 2, pp. 1–18, Jun. 2024, doi: 10.3897/aldj.2.117753.

[11] R. D. J. Iii, “NIST 101. Computational Chemistry Comparison and Benchmark Database,” *NIST*, Nov. 1999, Accessed: Feb. 13, 2025. [Online]. Available: https://www.nist.gov/publications/nist-101-computational-chemistry-comparison-and-benchmark-database

[12] None Available, “Materials Data on $P_4S_3$ by Materials Project.” LBNL Materials Project; Lawrence Berkeley National Laboratory (LBNL), Berkeley, CA (United States), 2020. doi: 10.17188/1190833.

[13] S. Shiotani, K. Ohara, H. Tsukasaki, S. Mori, and R. Kanno, “Pair distribution function analysis of sulfide glassy electrolytes for all-solid-state batteries: Understanding the improvement of ionic conductivity under annealing condition,” *Sci Rep*, vol. 7, no. 1, p. 6972, Aug. 2017, doi: 10.1038/s41598-017-07086-y.

[14] None Available, “Materials Data on $Li_2O$ by Materials Project.” LBNL Materials Project; Lawrence Berkeley National Laboratory (LBNL), Berkeley, CA (United States), 2020. doi: 10.17188/1194803.
[15] None Available, “Materials Data on GeS by Materials Project.” LBNL Materials Project; Lawrence Berkeley National Laboratory (LBNL), Berkeley, CA (United States), 2020. doi: 10.17188/1197633.
